# Supplementary material for: ORMA: Optimization-based Monocular 4D Reconstruction of Articulated Animals
Source: arXiv:2609.37986 source file (2026-09-29)
Supplement: Supplementary file 3 [file 03_more_results.tex]

In this section we present additional qualitative results that complement the experiments reported in the main paper. These examples include further comparisons with concurrent methods, additional animal categories, limitations, and results on real video sequences from the COP3D \cite{sinha2022common} and Pferd \cite{Li2024PFERD} datasets.

To facilitate navigation through the supplementary material, we organize the results as follows:

\begin{itemize}
\item Method comparisons: pages 6--12
\item Additional animal categories: pages 13--16
\item Real-world videos (COP-3D and Pferd): pages 17--26
\end{itemize}

Each page contains several representative examples illustrating the robustness of our approach across different animal species, poses, and video conditions.

\subsection{Limitations and Failure Cases}
Our approach is subject to several limitations arising from the underlying model assumptions and the reconstruction pipeline.
\vspace{0.4cm}\\
First, some errors originate from limitations in the SMAL fitting process when representing certain pose variations present in real animals. Although the SMAL model is capable of representing ear articulation and mouth opening, in practice these degrees of freedom are often not properly recovered during optimization. Instead of activating the corresponding articulations, the optimizer may compensate by fitting the ears inside the silhouette or by positioning the mouth in regions where the silhouette is wider, sometimes leaving the jaw contour mismatched. Similarly, the model struggles to accurately represent seated poses, where the animal’s limbs and body undergo strong articulation and contact with the ground. Finally, errors may arise during the alignment between SMAL and Hunyuan3D meshes. When the two geometries differ significantly, the registration step can become unstable and produce an inaccurate final shape.


\begin{figure}
    \centering
    \includegraphics[width=1\linewidth]{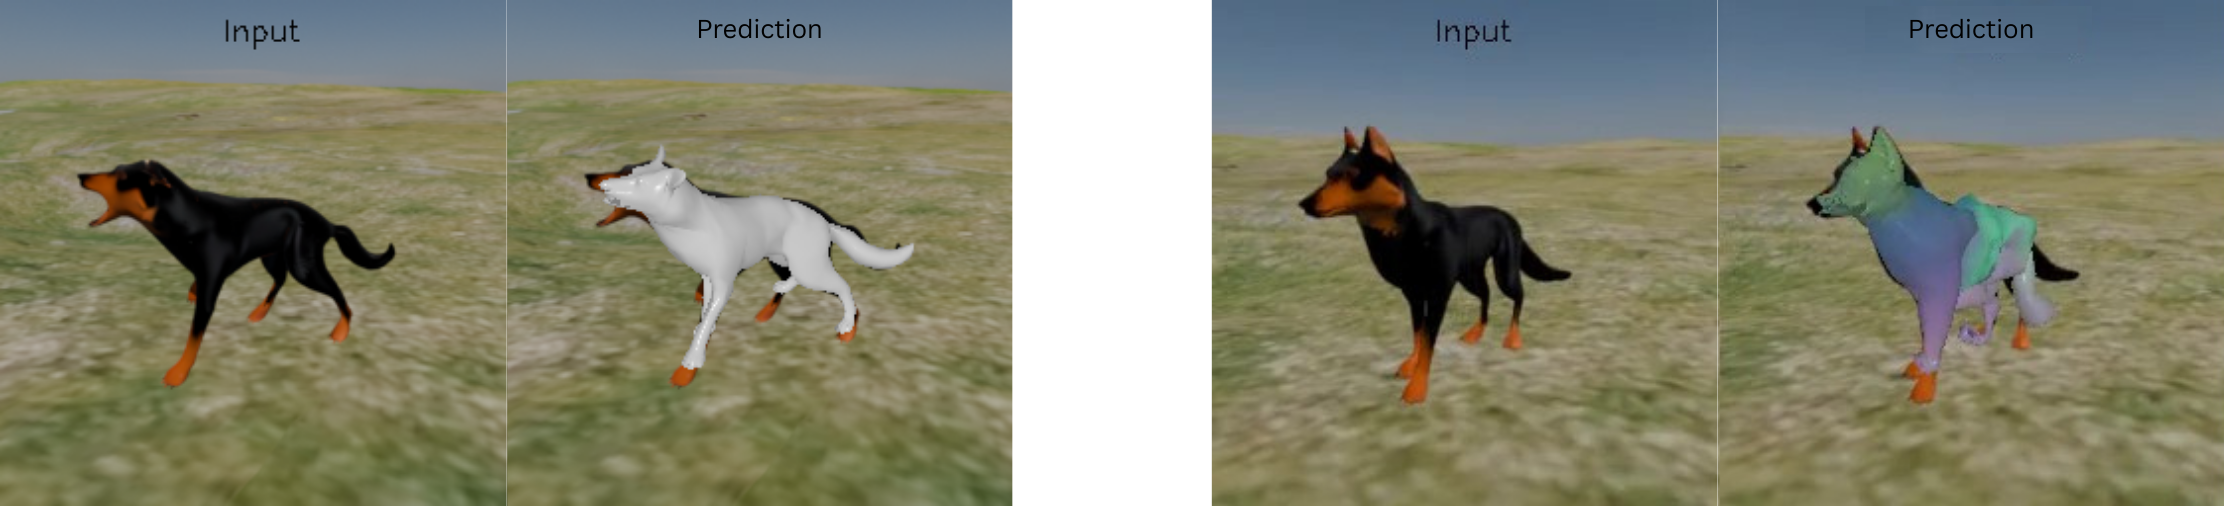}
    \caption{Examples of failure cases. Left: errors in the SMAL fitting process when the animal opens its mouth. Although SMAL can represent mouth articulation, the optimization sometimes fails to recover it, leading to incorrect silhouette alignment. Right: Hun3D mesh registration failure caused by significant geometric differences between the meshes.}
    \label{fig:fail}
\end{figure}

\newpage
\subsection{More Comparisons}

\begin{figure}[H]
    \centering
    \includegraphics[width=1\linewidth]{figures/results/comp1.png}
\end{figure}
\begin{figure}[H]
    \centering
    \includegraphics[width=1\linewidth]{figures/results/comp2.png}
\end{figure}
\begin{figure}[H]
    \centering
    \includegraphics[width=1\linewidth]{figures/results/comp3.png}
\end{figure}
\begin{figure}[H]
    \centering
    \includegraphics[width=1\linewidth]{figures/results/comp4.png}
\end{figure}
\begin{figure}[H]
    \centering
    \includegraphics[width=1\linewidth]{figures/results/comp5.png}
\end{figure}
\begin{figure}[H]
    \centering
    \includegraphics[width=1\linewidth]{figures/results/comp6.png}
\end{figure}
\begin{figure}[H]
    \centering
    \includegraphics[width=1\linewidth]{figures/results/comp7.png}
\end{figure}
\subsection{Other Animals}
\begin{figure}[H]
    \centering
    \includegraphics[width=1\linewidth]{figures/results/oa1.png}
\end{figure}
\begin{figure}[H]
    \centering
    \includegraphics[width=1\linewidth]{figures/results/oa2.png}
\end{figure}
\begin{figure}[H]
    \centering
    \includegraphics[width=1\linewidth]{figures/results/oa3.png}
\end{figure}
\begin{figure}[H]
    \centering
    \includegraphics[width=1\linewidth]{figures/results/oa4.png}
\end{figure}

\subsection{COP3D Results}
\begin{figure}[H]
    \centering
    \includegraphics[width=1\linewidth]{figures/results/cop1.png}
\end{figure}
\begin{figure}[H]
    \centering
    \includegraphics[width=1\linewidth]{figures/results/cop2.png}
\end{figure}
\begin{figure}[H]
    \centering
    \includegraphics[width=1\linewidth]{figures/results/cop3.png}
\end{figure}
\begin{figure}[H]
    \centering
    \includegraphics[width=1\linewidth]{figures/results/cop4.png}
\end{figure}
\begin{figure}[H]
    \centering
    \includegraphics[width=0.8\linewidth]{figures/results/cop5.png}
\end{figure}
\begin{figure}[H]
    \centering
    \includegraphics[width=0.8\linewidth]{figures/results/cop6.png}
\end{figure}
\begin{figure}[H]
    \centering
    \includegraphics[width=0.8\linewidth]{figures/results/cop7.png}
\end{figure}
\begin{figure}[H]
    \centering
    \includegraphics[width=0.8\linewidth]{figures/results/cop8.png}
\end{figure}

\subsection{PFERD Results}
\begin{figure}[H]
    \centering
    \includegraphics[width=1\linewidth]{figures/results/PFERD1.png}
\end{figure}
\begin{figure}[H]
    \centering
    \includegraphics[width=1\linewidth]{figures/results/PFERD2.png}
\end{figure}
